# Supplementary material for: Scaling Up Distance-generalized Core Decomposition
Source: arXiv:2006.03372 source file (2021-10-22)
Supplement: Supplementary file 1 [file supdoc.tex]

\begin{figure*}[t!]\vspace*{-0.6cm}
	\begin{center}
		\begin{tabular}[t]{c}\hspace*{-0.3cm}
			\subfigure[{\scriptsize $h=2$, top-$1$}]{
				\includegraphics[width=0.45\columnwidth, height=2.5cm]{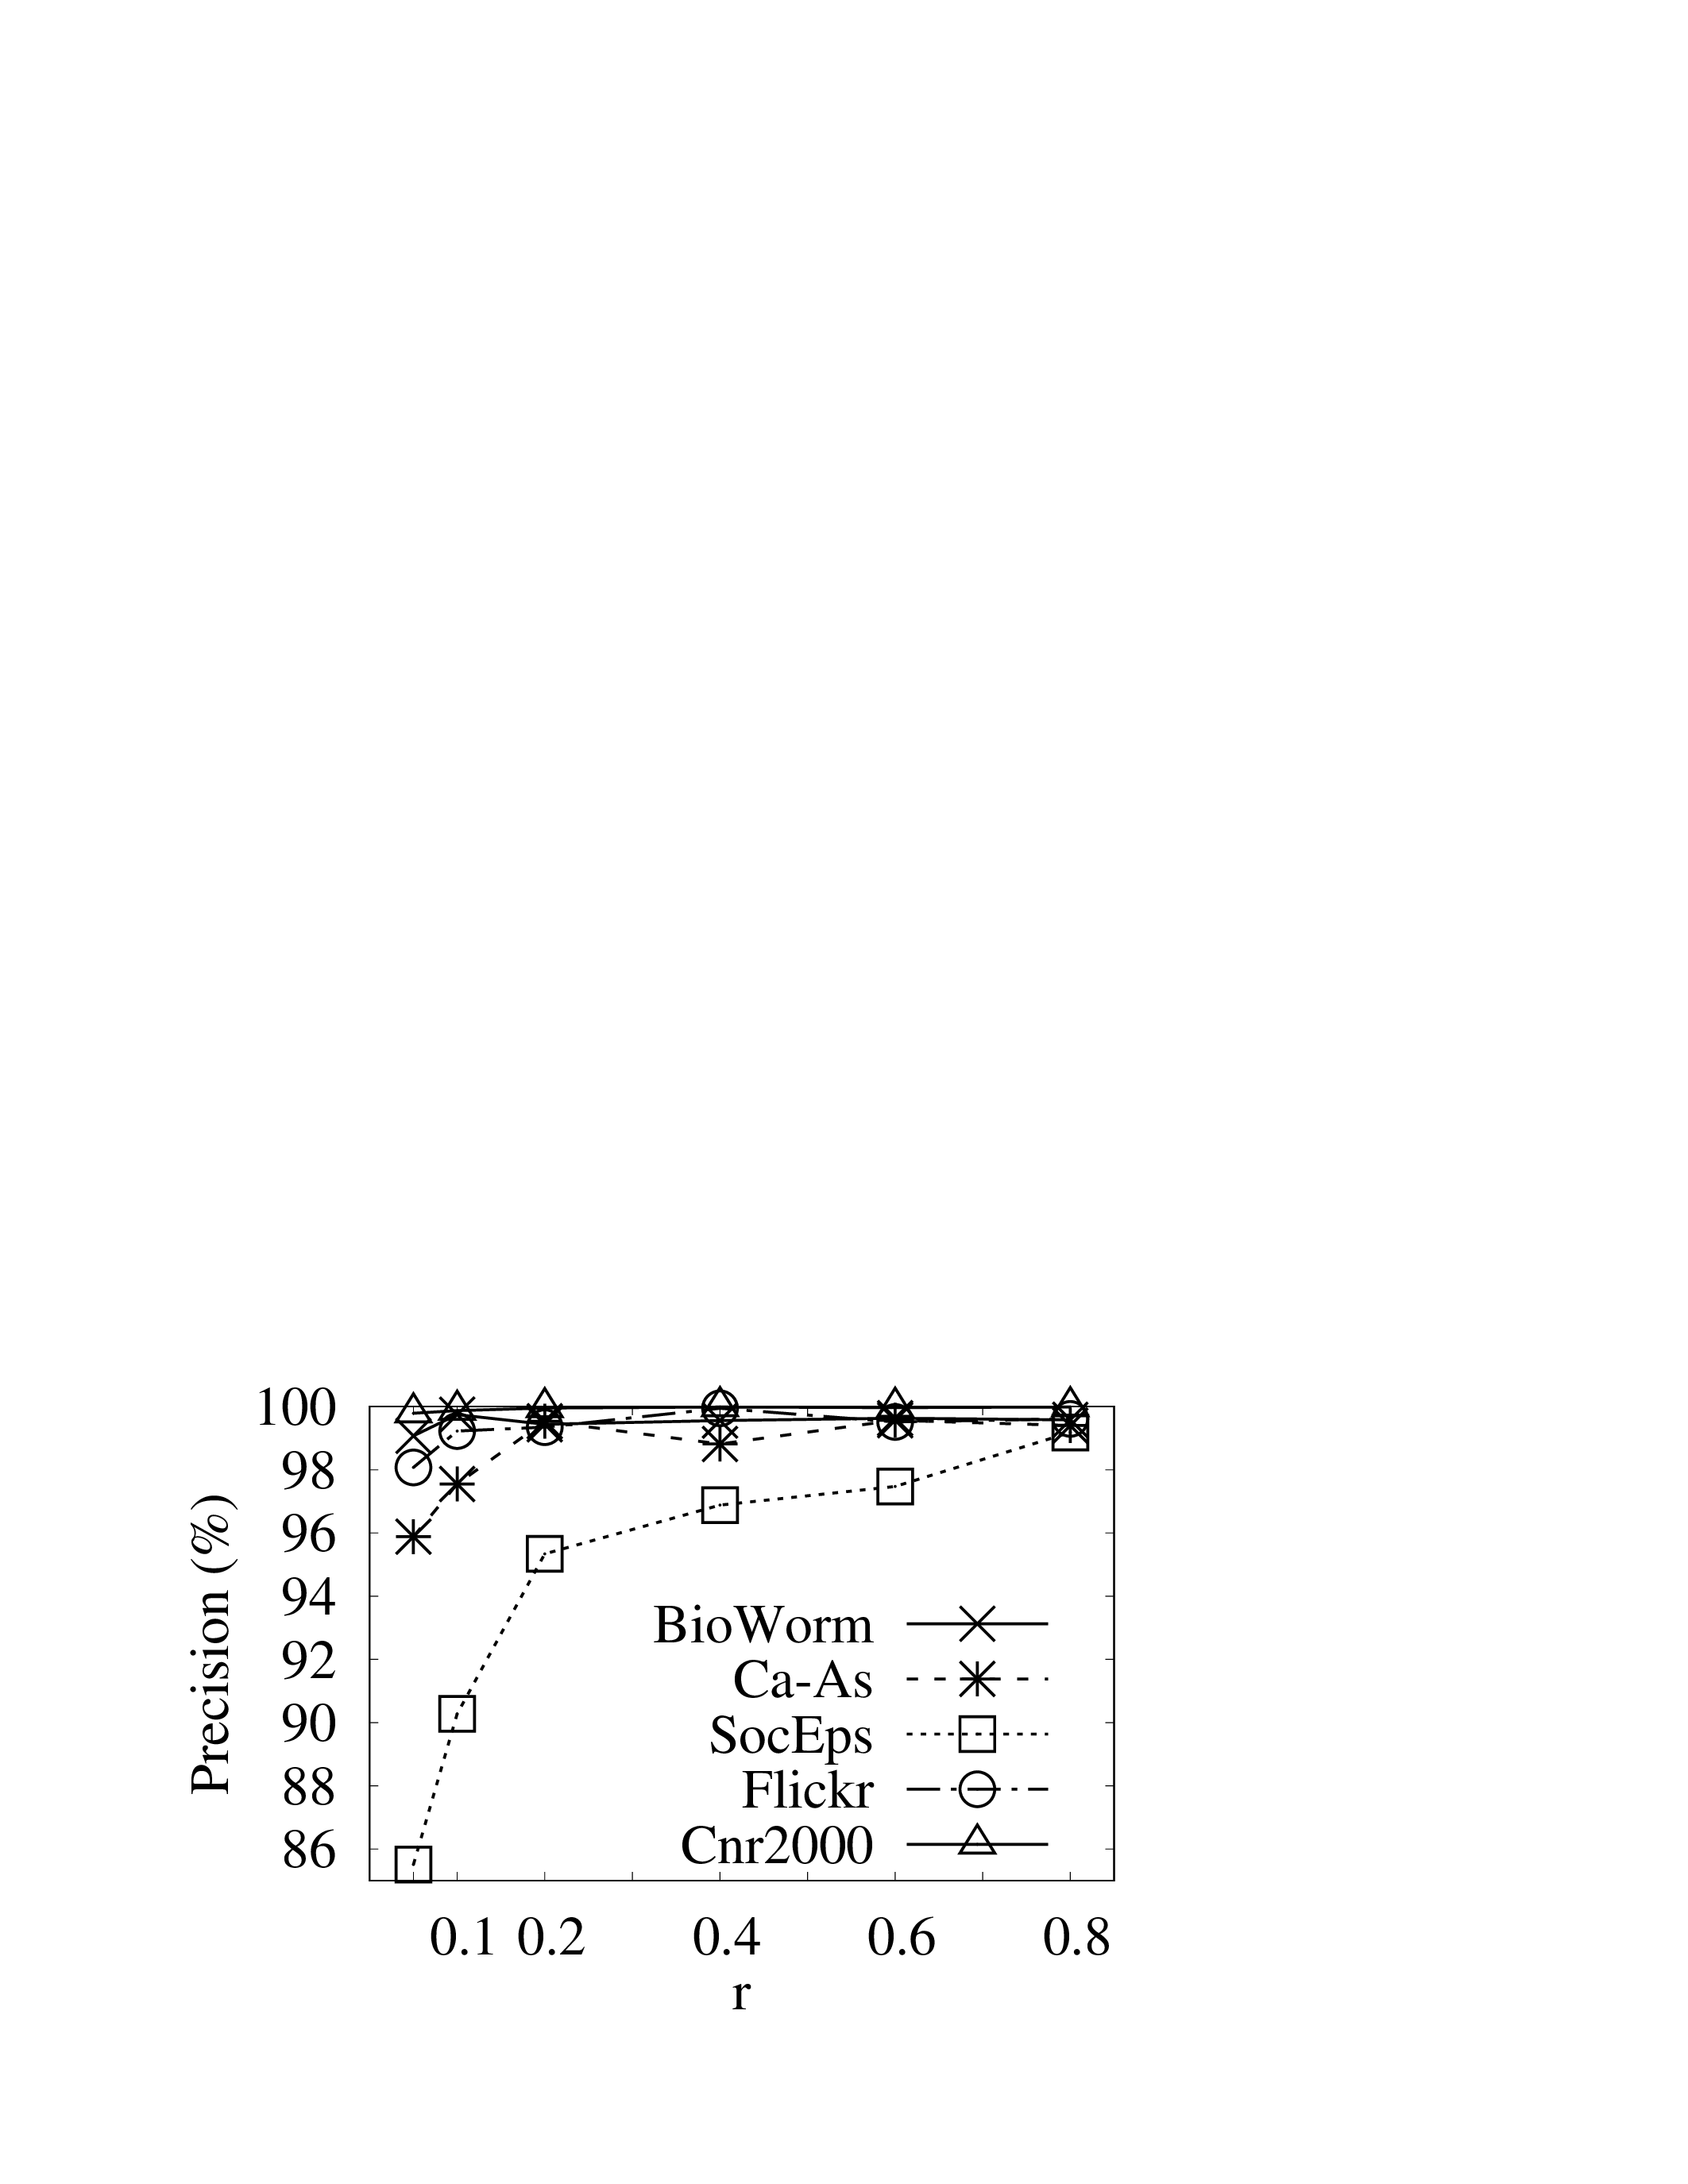}
			}\hspace*{0.3cm}
			\subfigure[{\scriptsize $h=3$, top-$1$}]{
				\includegraphics[width=0.45\columnwidth, height=2.5cm]{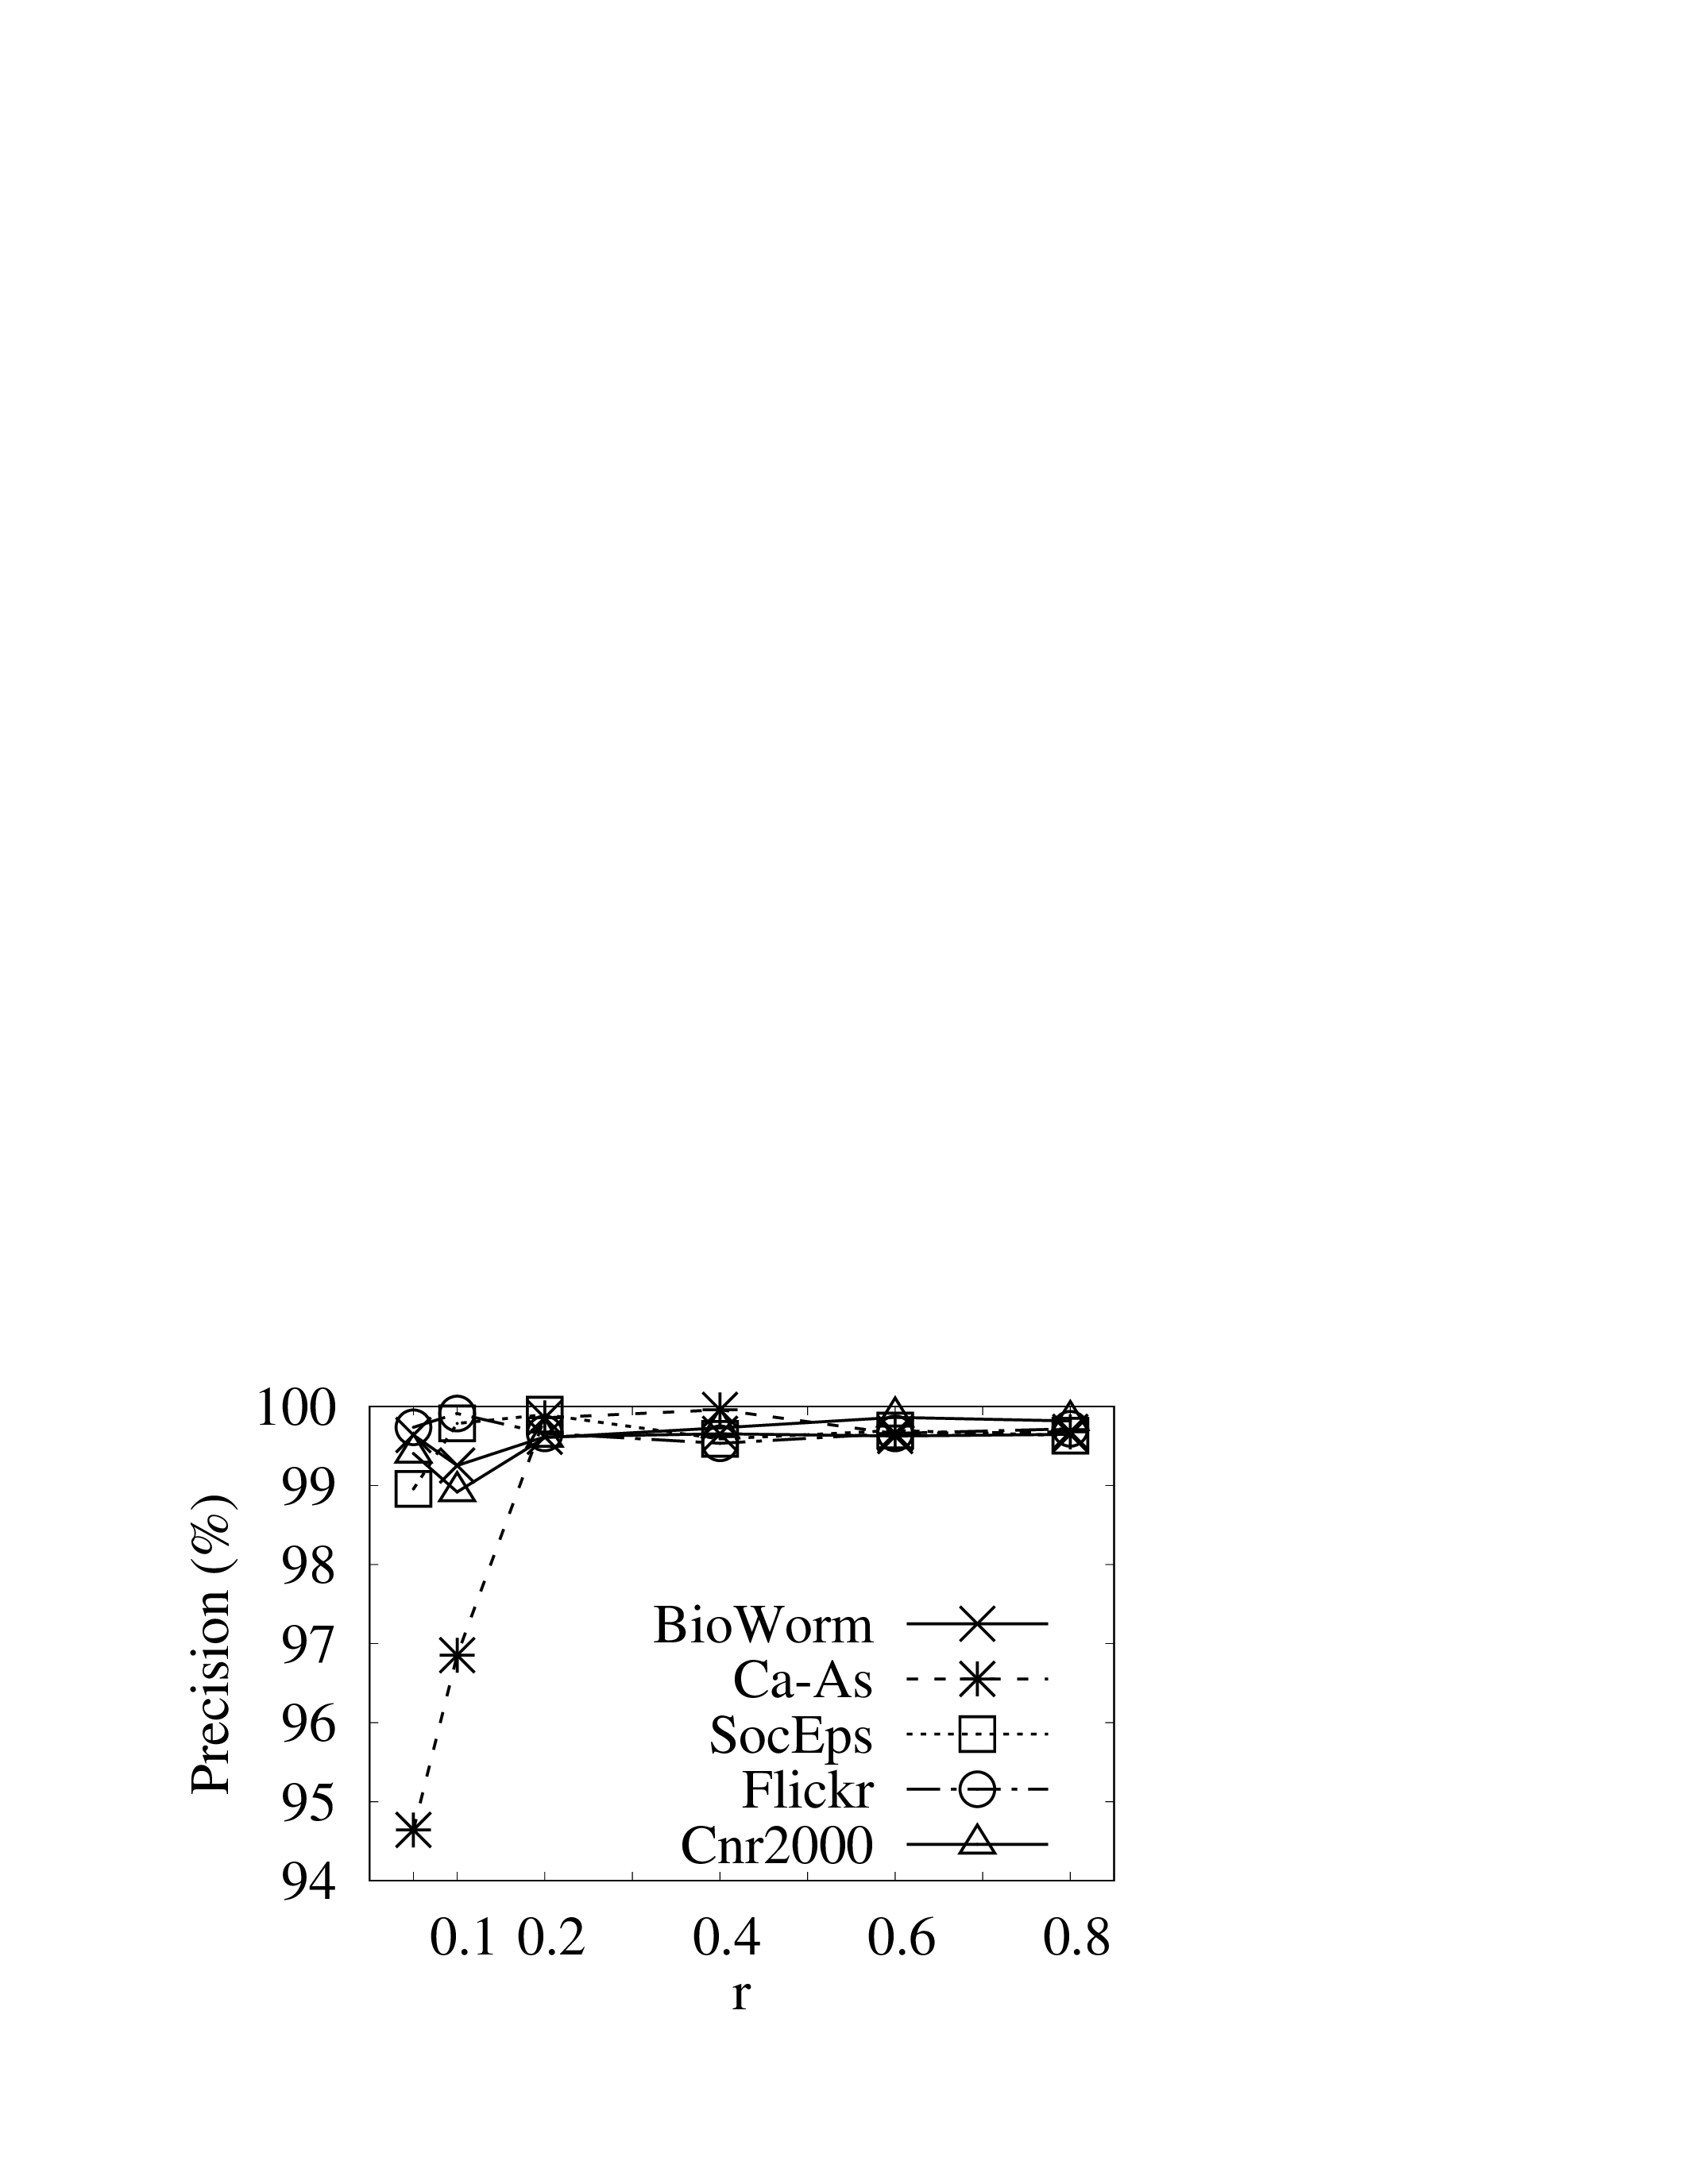}
			}\hspace*{0.3cm}
			\subfigure[{\scriptsize $h=4$, top-$1$}]{
				\includegraphics[width=0.45\columnwidth, height=2.5cm]{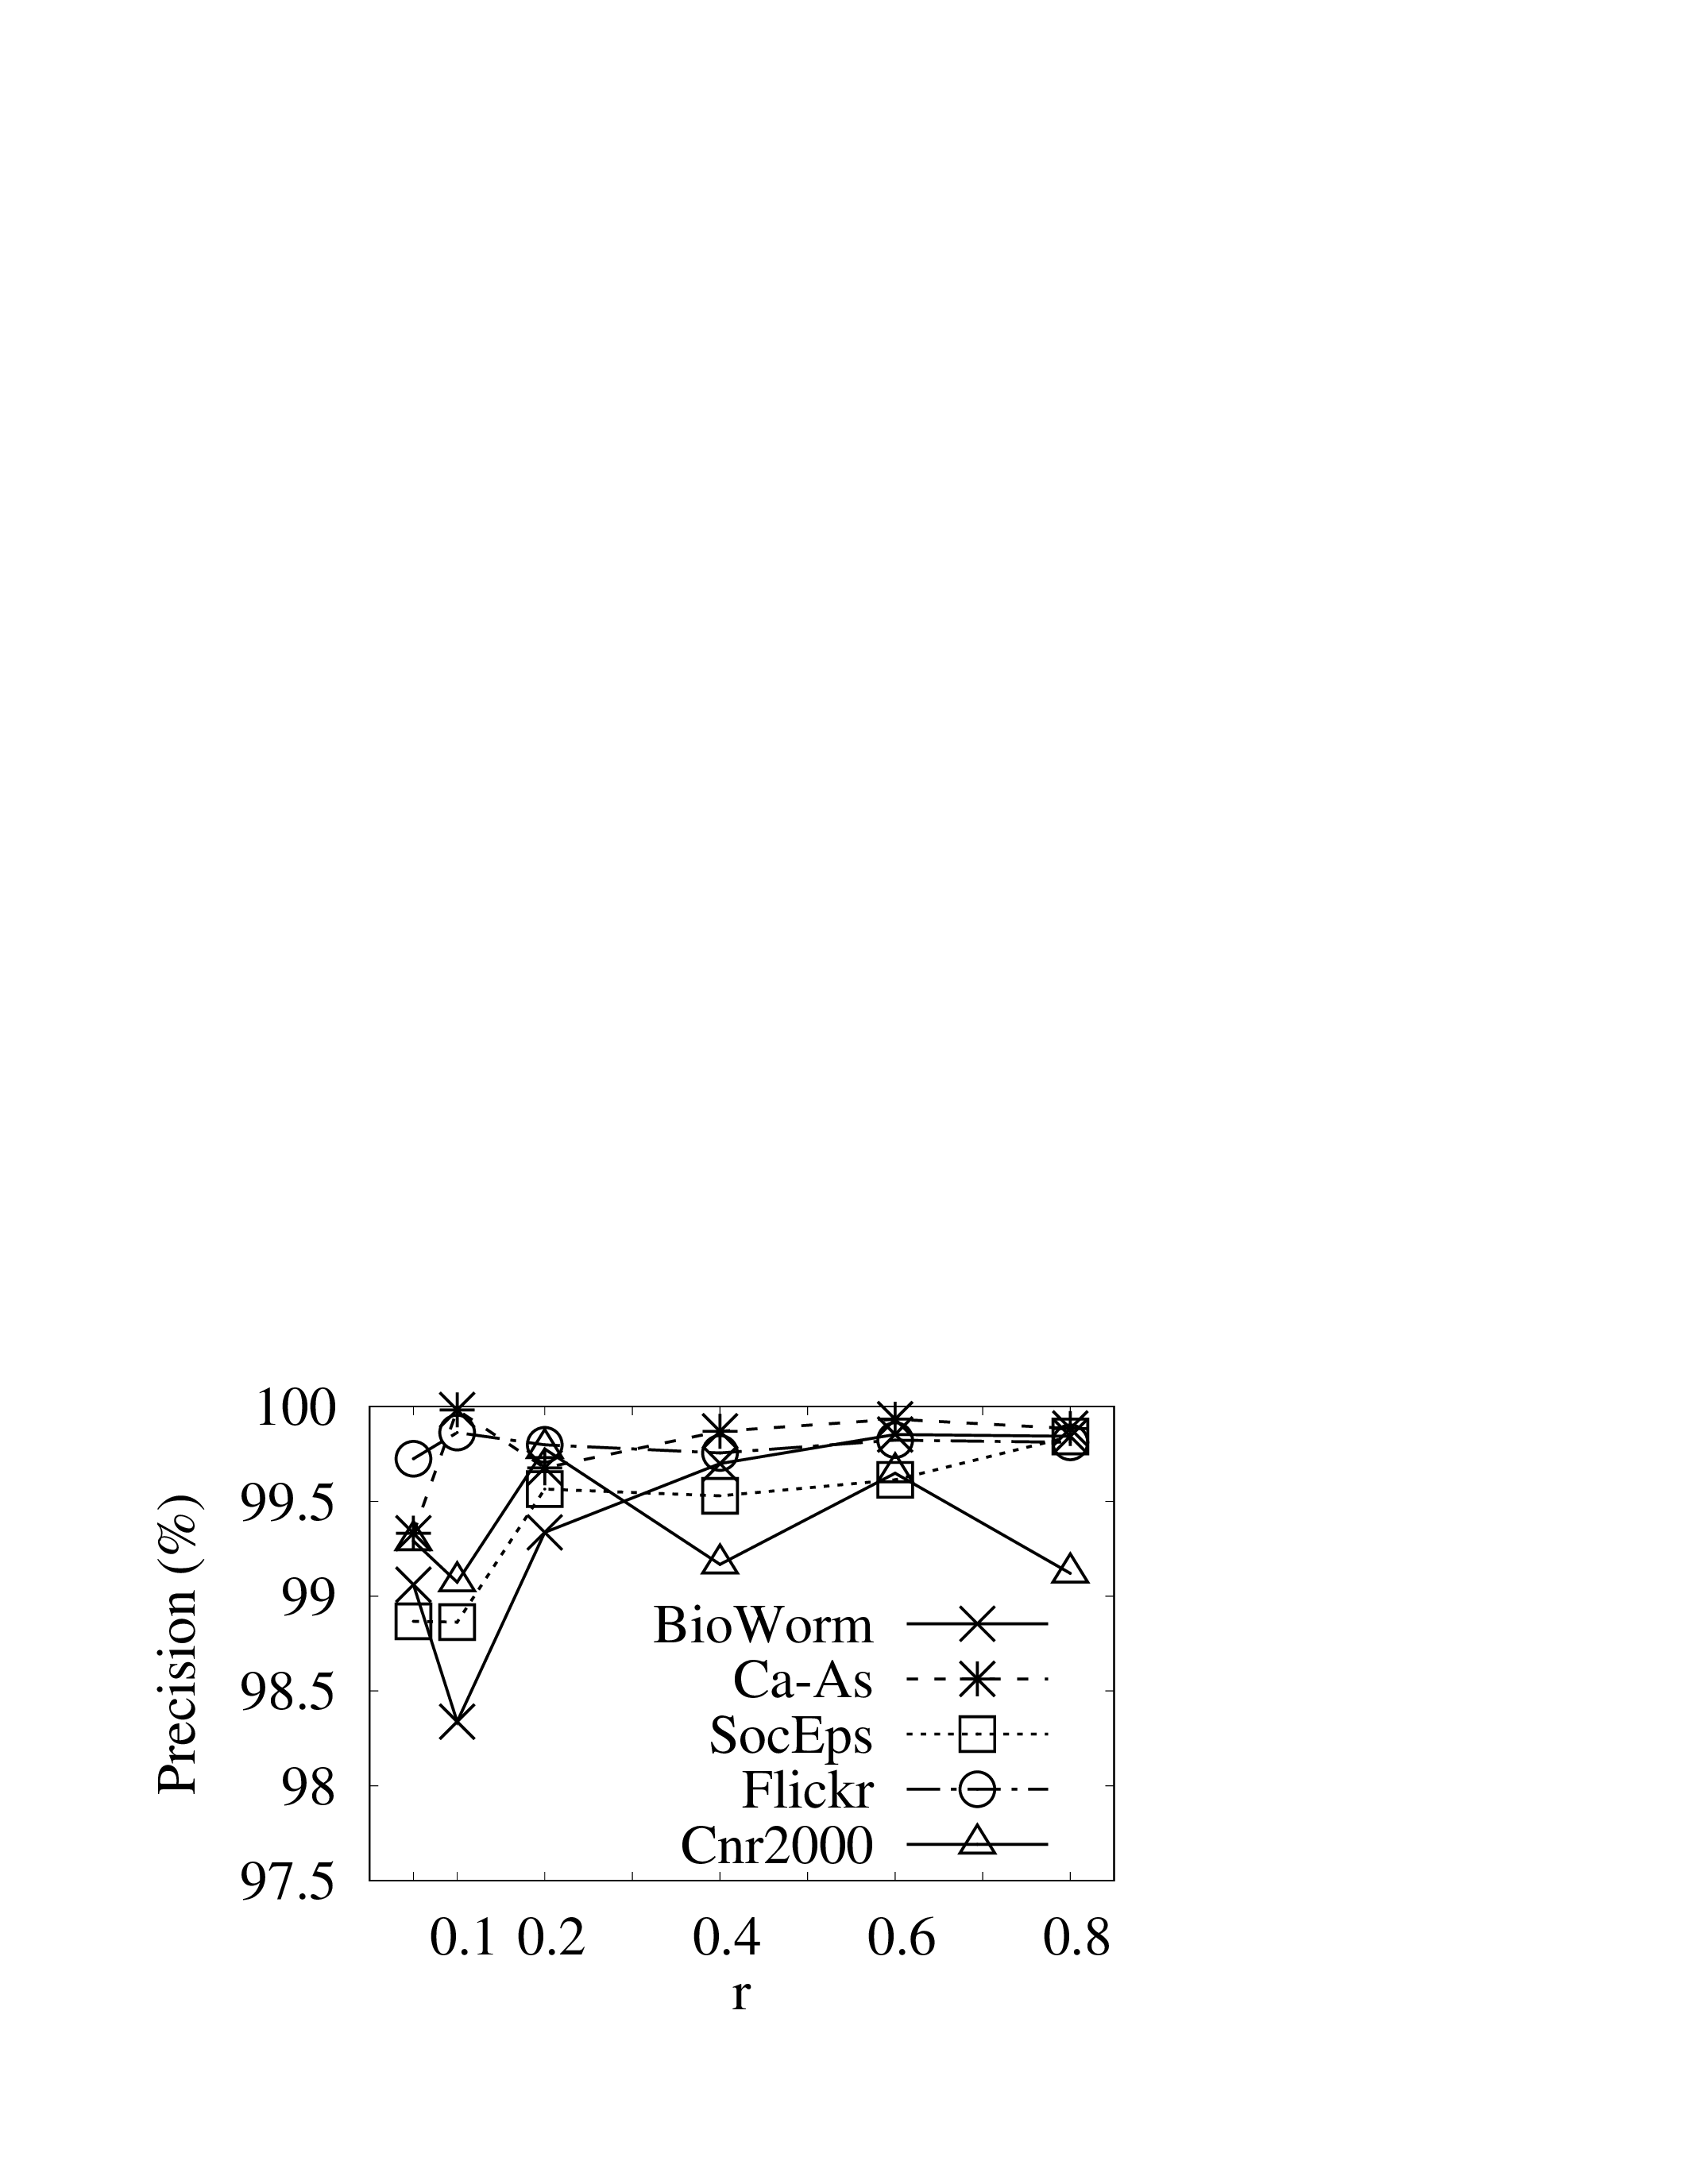}
			}\hspace*{0.3cm}
			\subfigure[{\scriptsize $h=5$, top-$1$}]{
				\includegraphics[width=0.45\columnwidth, height=2.5cm]{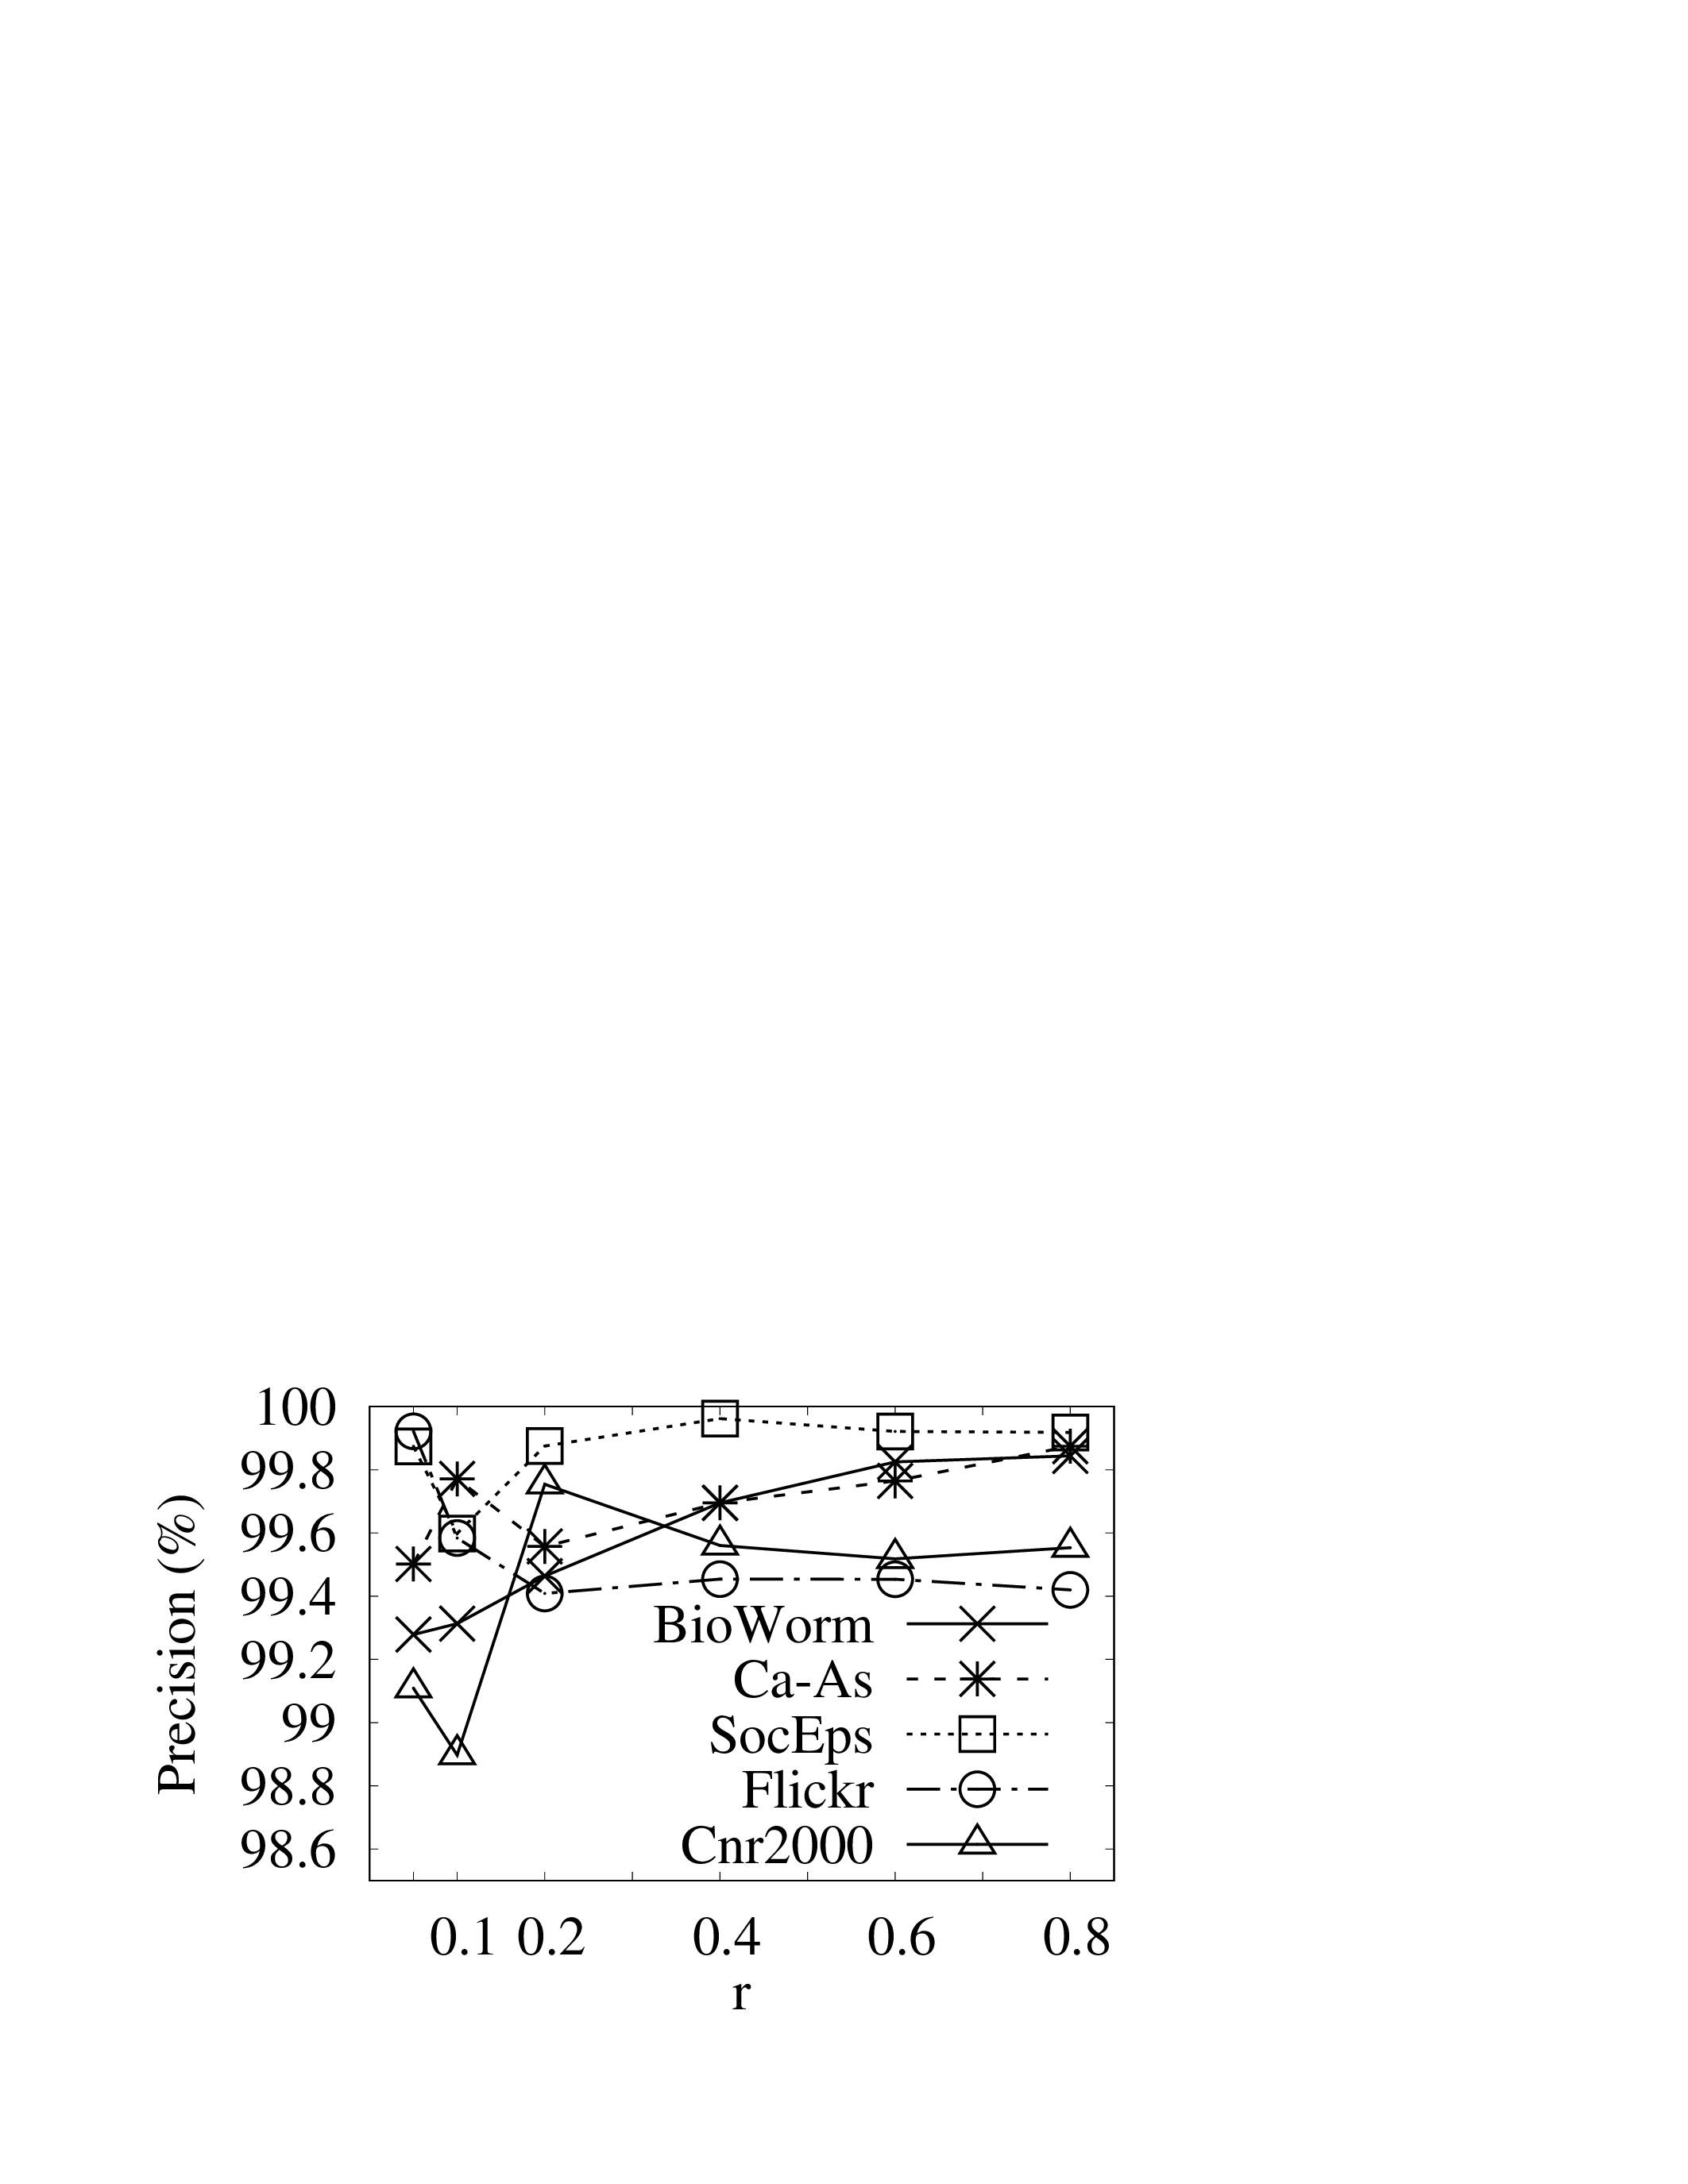}
			}
\vspace*{-0.35cm}\\ \hspace*{-0.3cm}
			\subfigure[{\scriptsize $h=2$, top-$50$}]{
				\includegraphics[width=0.45\columnwidth, height=2.5cm]{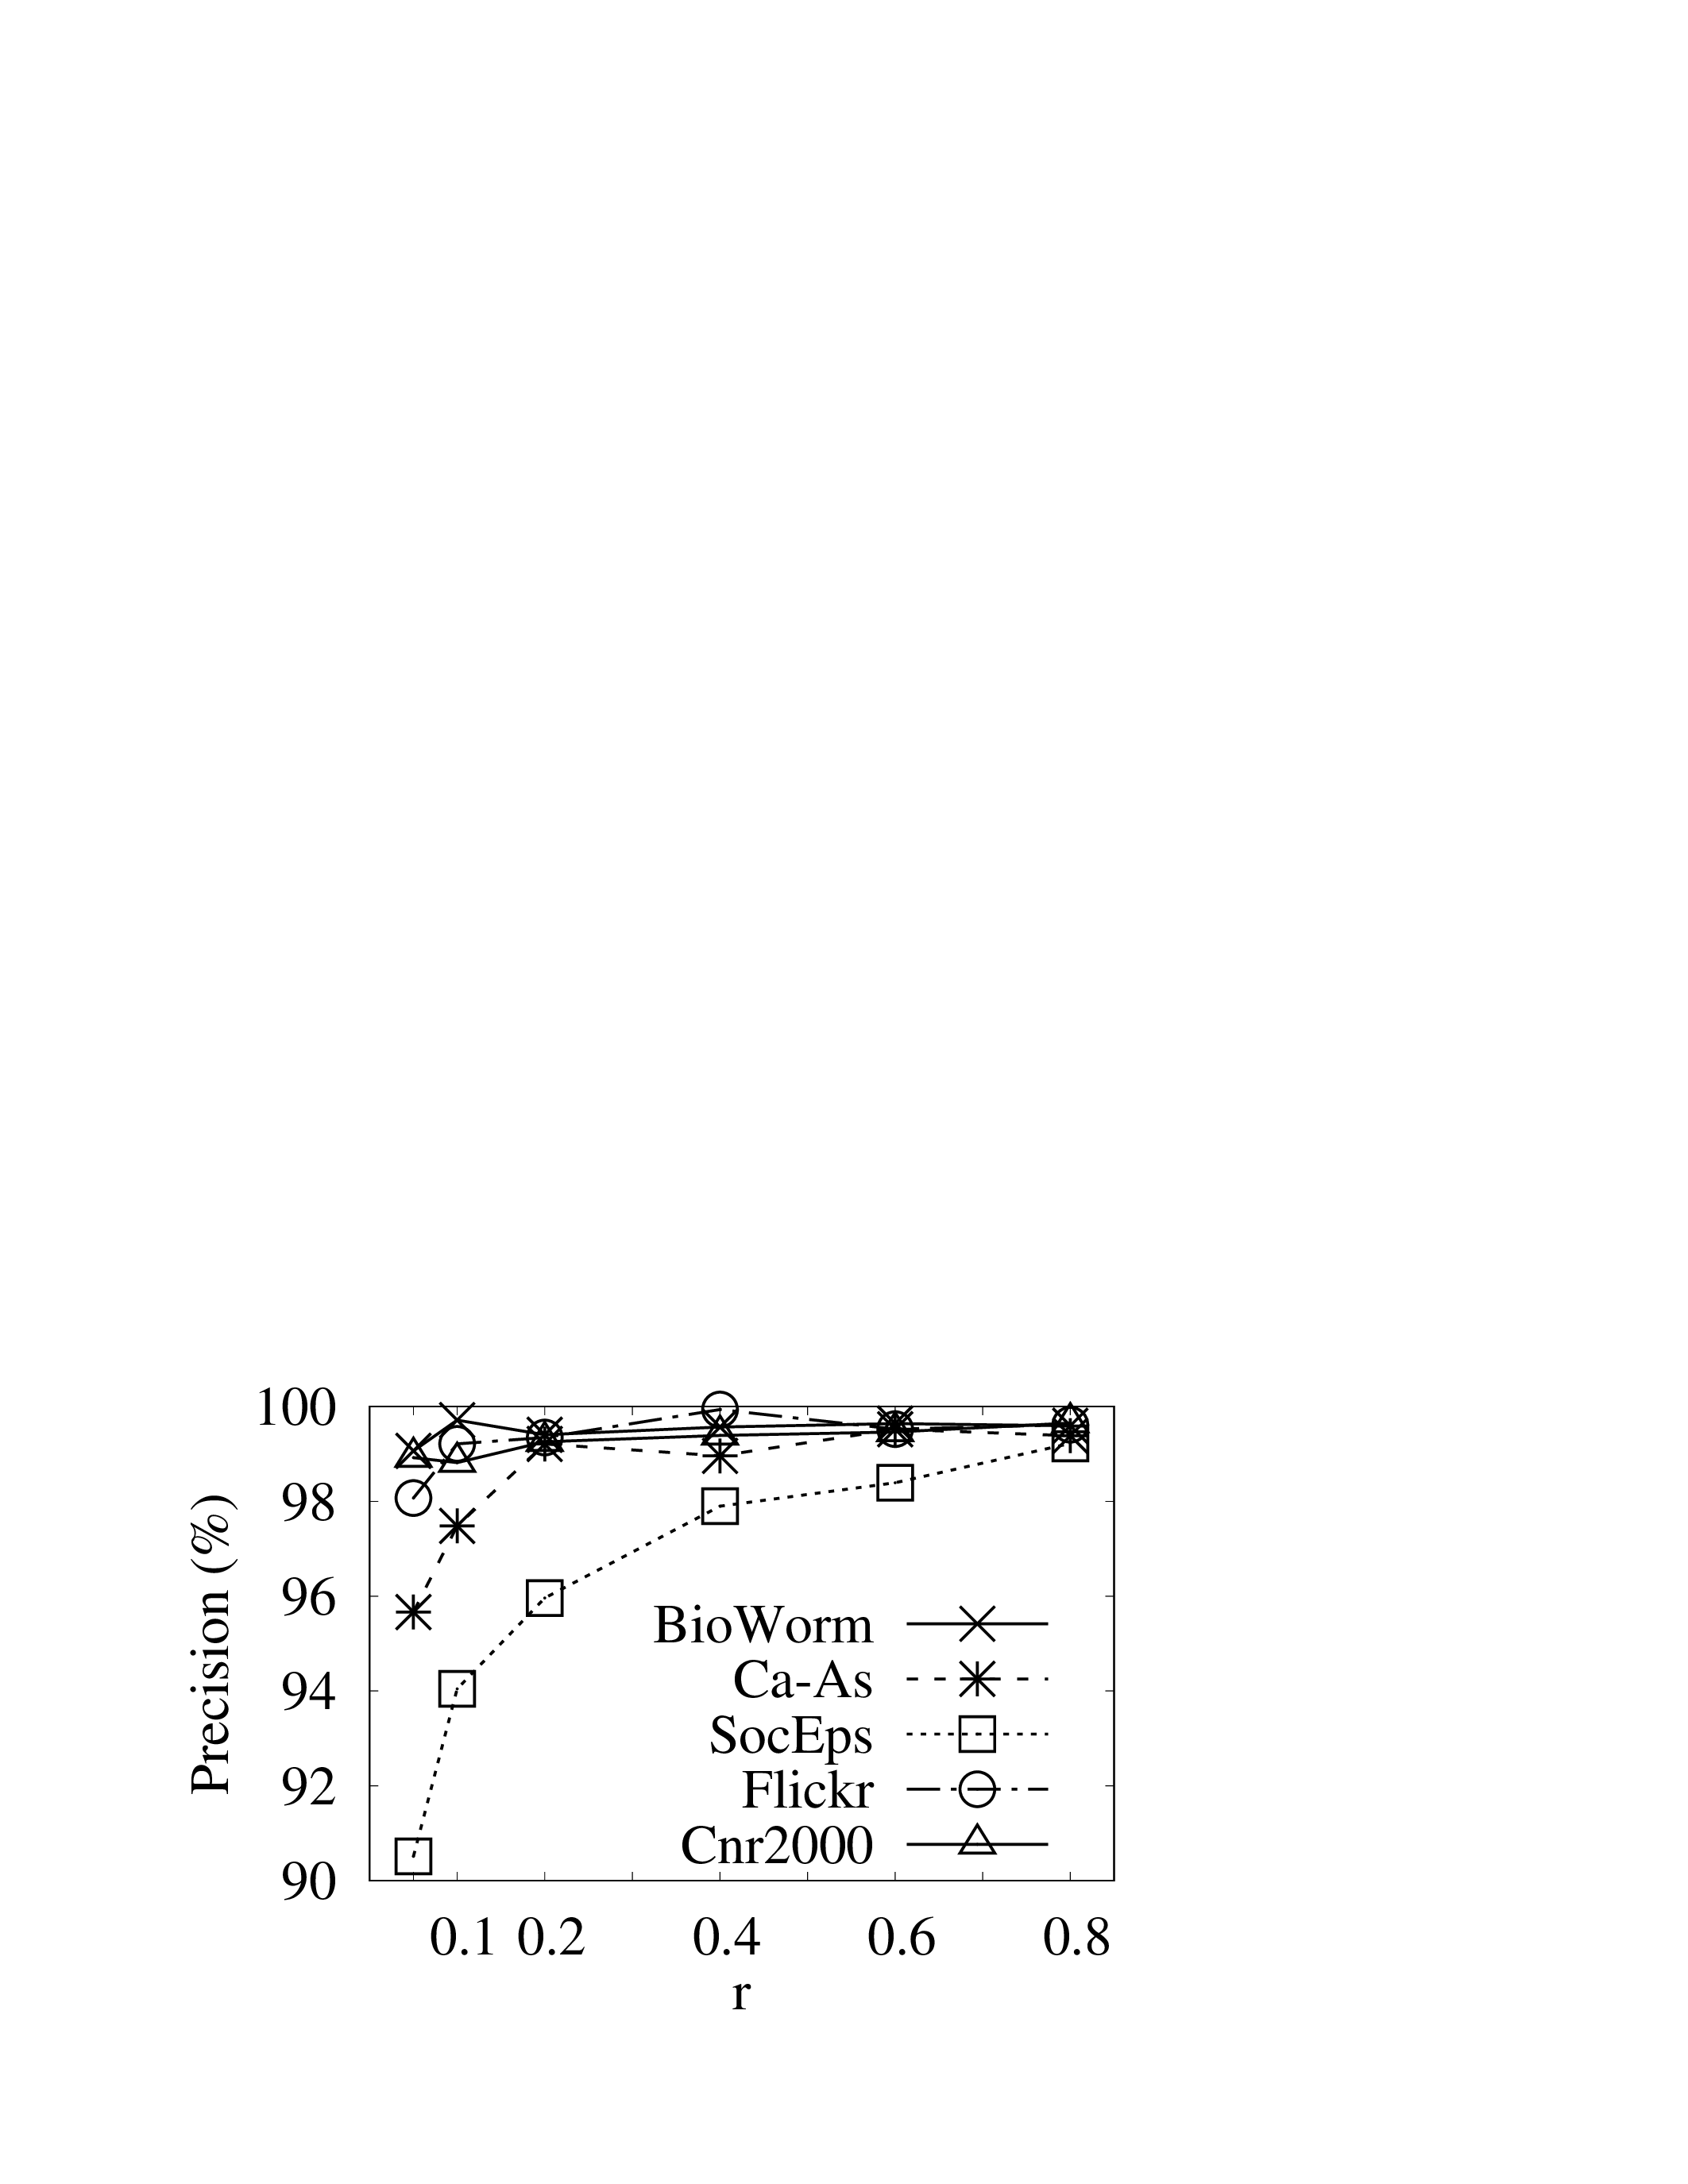}
			}\hspace*{0.3cm}
			\subfigure[{\scriptsize $h=3$, top-$50$}]{
				\includegraphics[width=0.45\columnwidth, height=2.5cm]{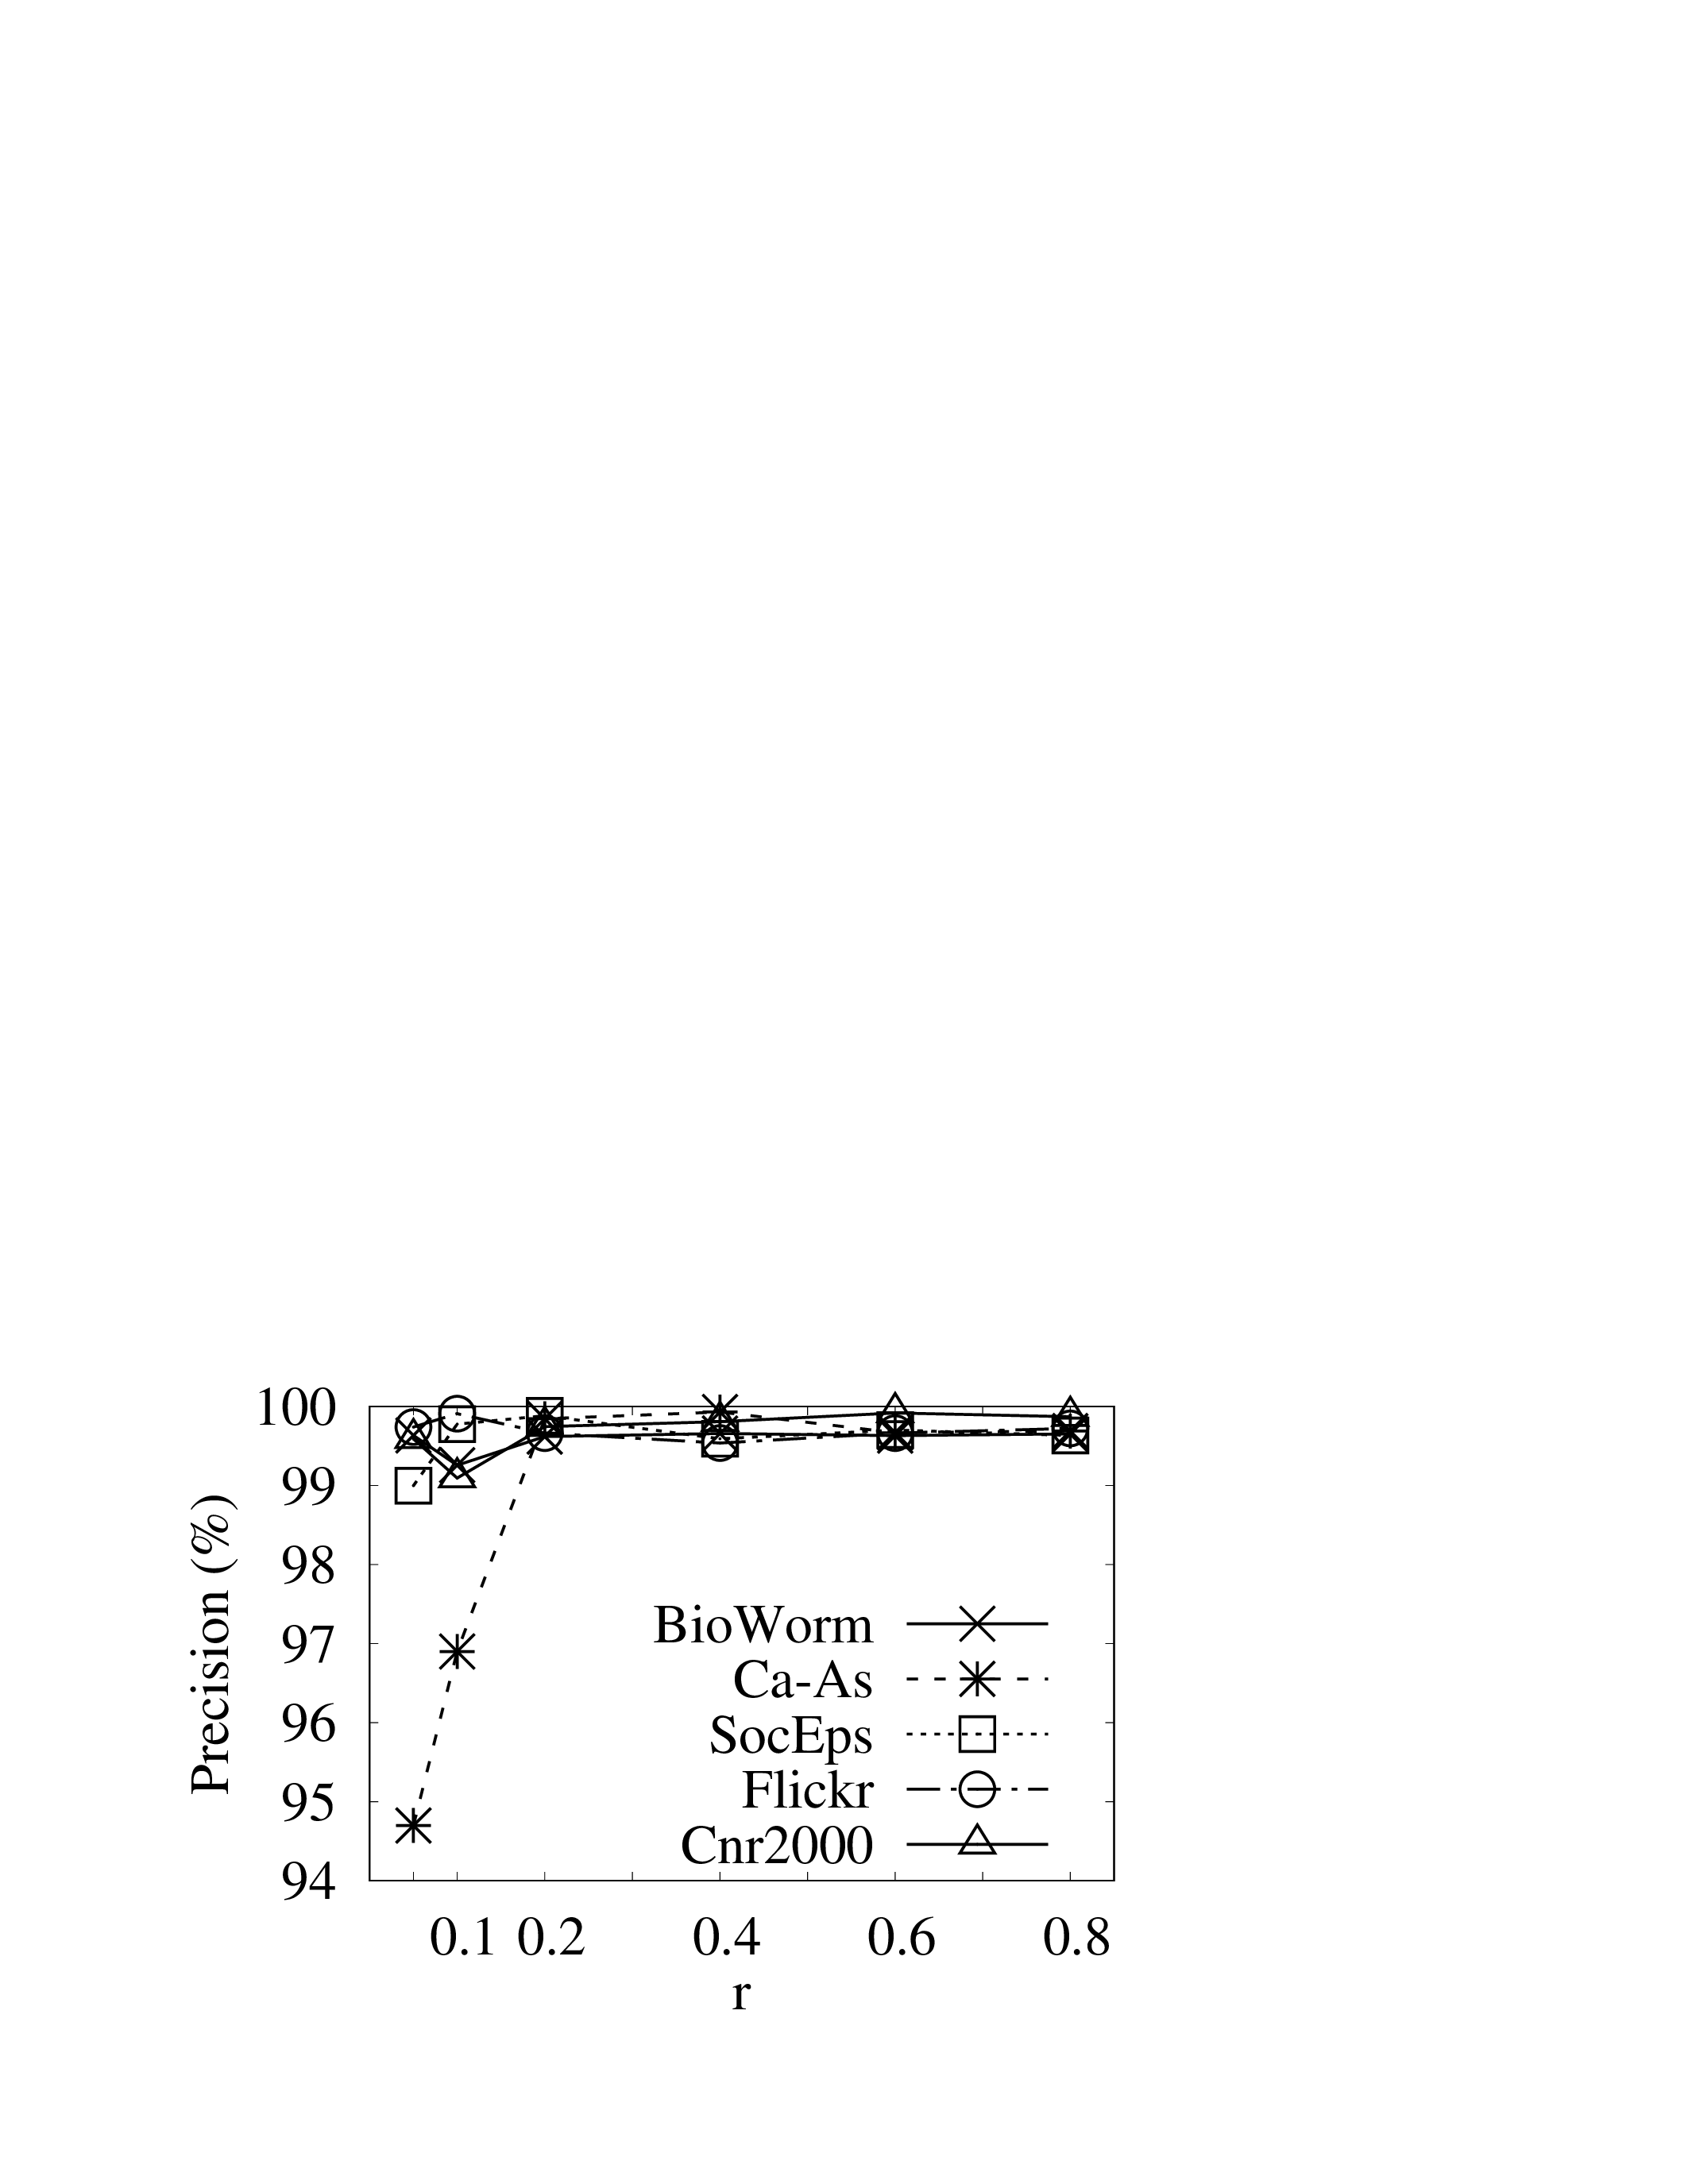}
			}\hspace*{0.3cm}
			\subfigure[{\scriptsize $h=4$, top-$50$}]{
				\includegraphics[width=0.45\columnwidth, height=2.5cm]{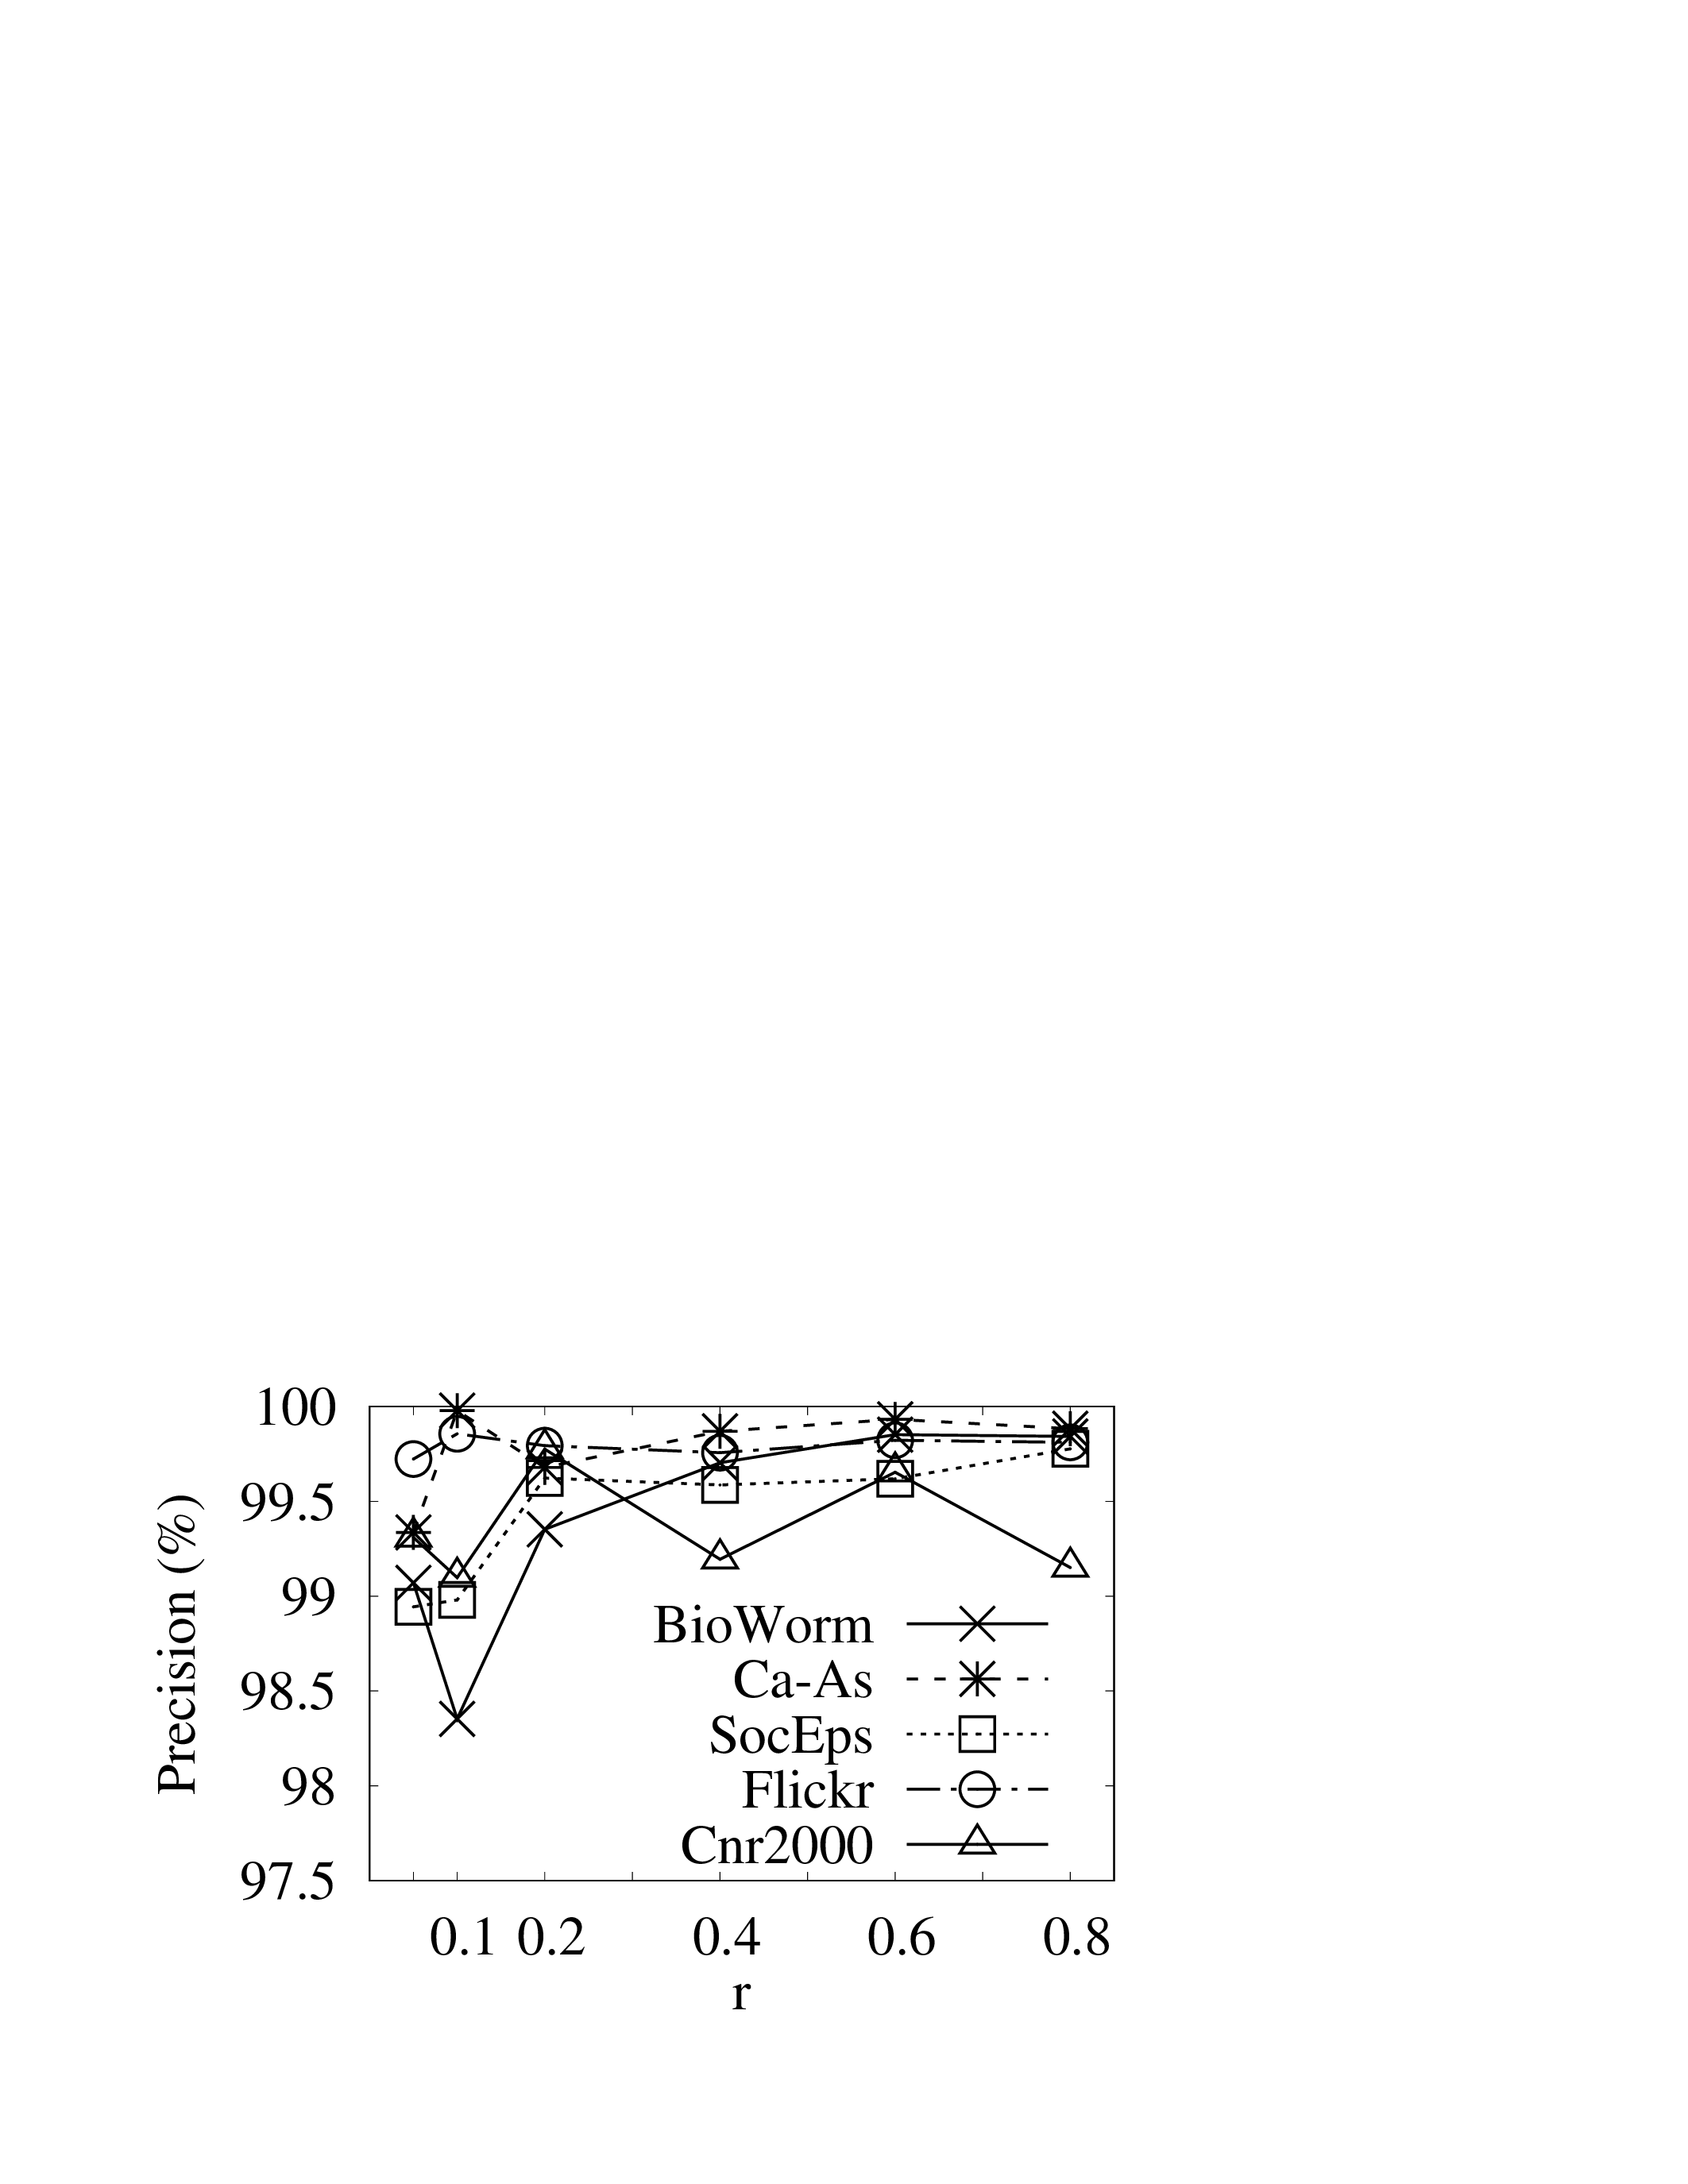}
			}\hspace*{0.3cm}
			\subfigure[{\scriptsize $h=5$, top-$50$}]{
				\includegraphics[width=0.45\columnwidth, height=2.5cm]{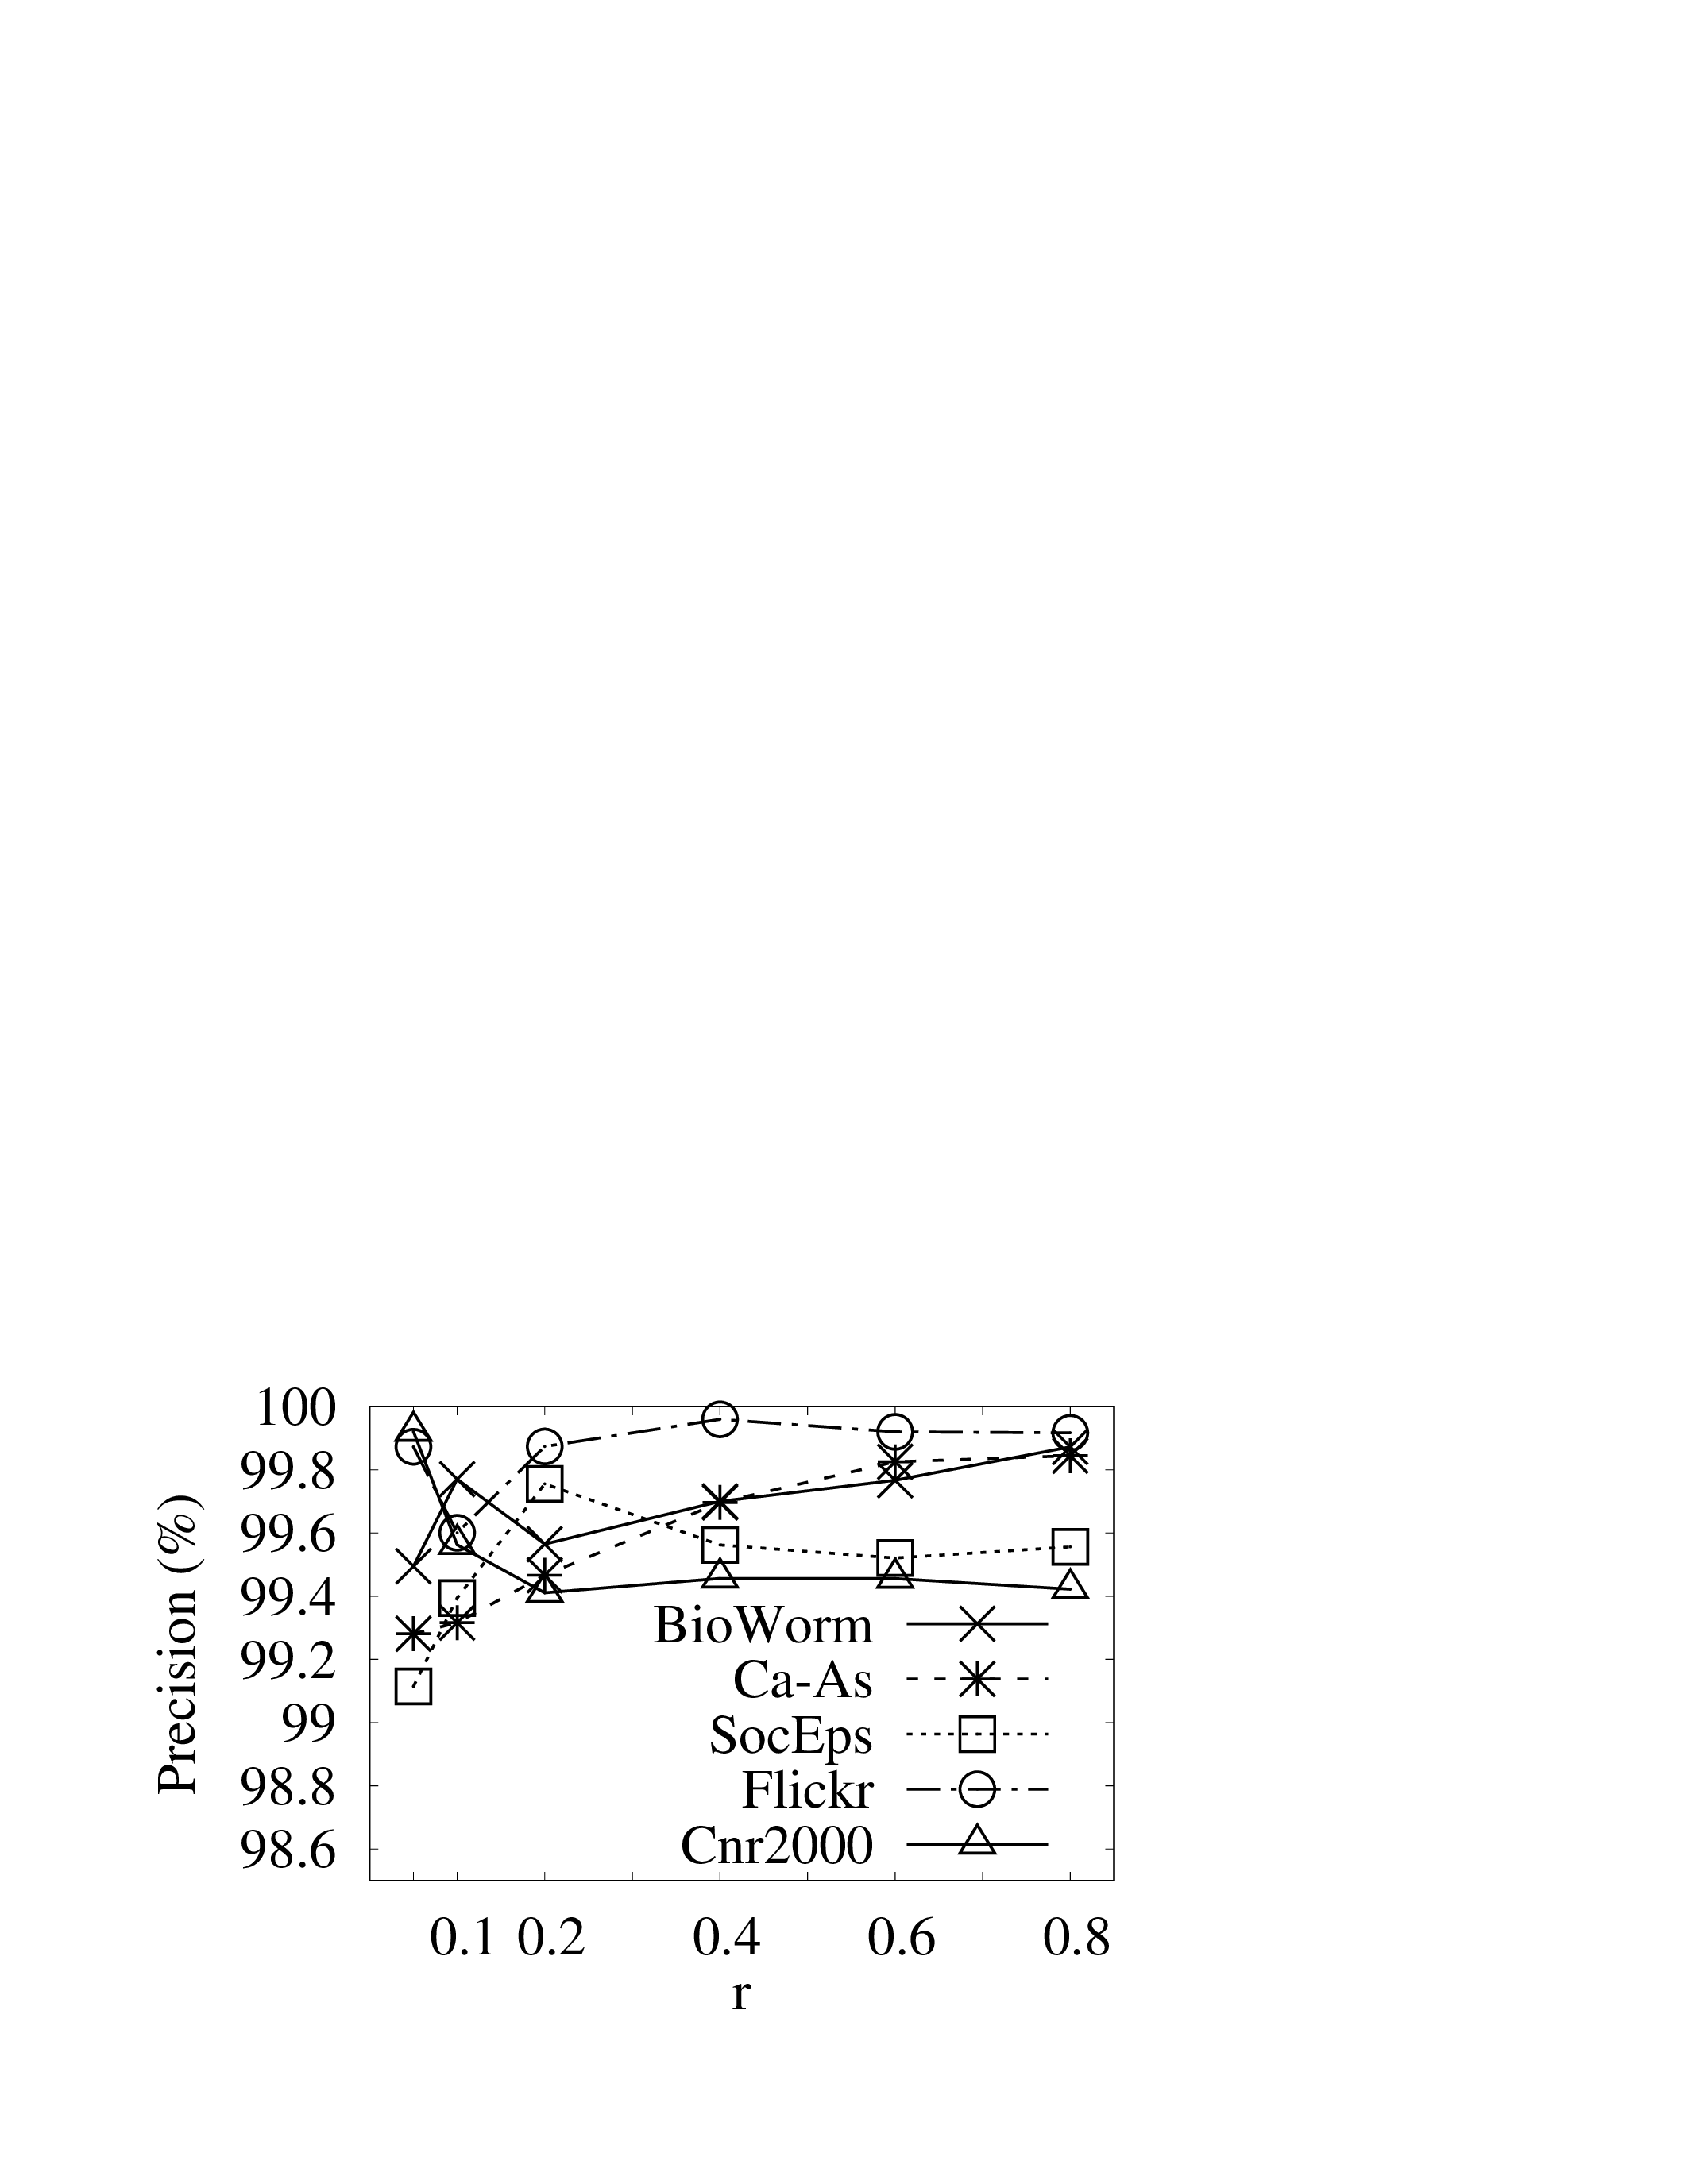}
			}
		\end{tabular}
	\end{center}
	\vspace*{-0.55cm}
	\caption{ Precisions of \khcs by only considering the top-$s$ maximal $(k,h)$-cores ($s=1$ and $s=50$)}
	\vspace*{-0.35cm}
	\label{fig:exp3:precision-vary-h-top-s}
\end{figure*}

\section{Supplemental Materials}
\label{sec:supple}

\vspace*{-0.1cm}
\subsection{Reproducibility}
For reproducibility purpose, the source code of this paper is released at an anonymous source \url{https://tinyurl.com/y2nu75jf}.
A ``readme" file is also included in our released source code package. Following the ``readme" file, one can easily compile and run our code.  All datasets used in our experiments are publicly available, and the results shown in this paper can be reproduced by running our code on these datasets.

%Note that all datasets used in the experiments are publicly available, thus we believe that the results shown in this paper can be easily reproduced.

\setcounter{section}{8}
\vspace*{-0.1cm}
\subsection{Additional Experiment}
In this experiment, we evaluate the precision of the \khcs algorithm by only considering the top-$s$ maximal $(k,h)$-cores. Specifically,  let  $\core_h[v]$ and $\widehat \core_h[v]$ be the exact and the estimated $(k,h)$-core number of the vertex $v$, respectively. Then, the precision of an algorithm is computed by $1-(\sum\nolimits_{v\in S}(|\core_h[v]-\widehat \core_h[v]|)/\core_h[v])/|S|$, where the $S$ is the set of vertices of the top-$s$ maximal $(k,h)$-cores. Fig.~\ref{fig:exp3:precision-vary-h-top-s} shows the precision results of \khcs on five datasets. Similar results can also be observed on the other datasets. As expected, the precisions of \khcs typically increase as $r$ increases on most datasets. When $h=2$ and $s=1$ (Fig.~\ref{fig:exp3:precision-vary-h-top-s}(a)), the precisions of \khcs are no less than 95\% on all datasets except \soceps even when $r=0.05$. Moreover, with $r$ increases, the precisions can be quickly improved to  98\% on most datasets given that $h=2$. When $h \geq 3$  (Fig.~\ref{fig:exp3:precision-vary-h-top-s}(b-d)), \khcs exhibits very high precisions ($\ge 99$\%) in most cases. From Fig.~\ref{fig:exp3:precision-vary-h-top-s}(e-h), we find that the results for $s=50$ are consistent. These results further confirm that the \khcs algorithm is very accurate in practice even for a very small sampling rate (e.g., $r=0.1$).

%Moreover, we can see that the precisions of \khcs slightly increase as $s$ increases.
\vspace*{-0.2cm}
\subsection{Missing Proofs}
\setcounter{observation}{0}
\begin{observation}
	\label{Obs:1}Given a positive integer $h \in \mathbb{N^{+}}$ and a vertex $u \in N_{v}^{h}(G) $, we have $S_u = N_u^{h}(G) \setminus (N_v^{h-s}(G) \cup \{v\}) \subseteq N_u^{h}(G(V\setminus\{v\}))$ for $s\le h$.
\end{observation}

\begin{proof}
Clearly, for any vertex $w \in S_u$, we have $dis_G(w,v) > h-s$ by definition. To prove the observation, we consider two disjoint subsets of $S_u$: $A=\{w|w\in S_u, dis_G(w,v)>h\}$ and $B=\{w|w\in S_u,h-s < dis_G(w,v)\leq h\}$. First, we claim that for any vertex $w \in A$, we have $w \in N_u^{h}(G(V\setminus\{v\}))$. Since $w\in S_u \subset N_u^h(G)$, we have $dis_G(w, u) \le h < dis_G(w, v)$. That is to say, there does not exist any shortest path between $u$ and $w$ that passes through $v$. Therefore, after deleting $v$ from $G$, the shortest-path distance between $w$ and $u$ does not affect, indicating that $dis_{G\setminus \{v\}}(w, u) \le h $. Second, for any vertex $w\in B$, we have $dis_G(u,w) < dis_G(u,v) + dis_G(v,w)$. This is because  $dis_G(u,w) \leq h$, $dis_G(u,v) = s $ and $dis_G(v,w) > h-s$. Therefore, any shortest-path between $u$ and $w$ does not pass through $v$, which suggests that $dis_{G(V\setminus \{v\})}(w, u) \le h $. %This completes the proof.
\end{proof}

\begin{observation}\label{Obs:2}
Given a positive integer $h \in \mathbb{N^{+}}$ and a vertex $u \in N_{v}^{h}(G) $, we define $\small F_u \triangleq \{w|w\in N_v^{h-s}(G), dis_{G(V\setminus \{v\})}(u,w)> h\}$. Then, we have $\small N_u^h(G) \setminus N_u^h(G(V\setminus\{v\}))= \{v\} \cup F_u$.
\end{observation}
\begin{proof}
  Clearly, the vertex $v$ is contained in $\small N_u^h(G) \setminus N_u^h(G(V\setminus\{v\}))$. On the one hand, for any vertex $w\ne v$ and $\small w  \in N_u^h(G) \setminus N_u^h(G(V\setminus\{v\}))$, we have $dis_{G}(u, w)\le h$ and $ dis_{G(V\setminus\{v\})}(u, w) $$>h $. Therefore, the shortest path from $u$ to $w$ in $G$ must pass through $v$. Since $dis_{G}(u, v) = s$, we have $dis_G(v, w) \le h-s$. In other words, $w \in N_v^{h-s}(G)$ which indicates that $w \in F_u$ holds. On the other hand, for any vertex  $w\ne v$ and $w \in F_u$, $w \notin N_u^h(G(V\setminus\{v\}))$ clearly holds (by the definition of $F_u$). Since $w\in N_v^{h-s}(G)$ and $dis_{G}(u, v) = s$, we have $dis_{G}(u, w) \le h$ by triangle inequality. Hence, we obtain that $w \in N_u^h(G)$. This completes the proof.
\end{proof}

\setcounter{section}{4}
\begin{theorem}
  \label{thm:h-neighbor} Given a positive integer $h \in \mathbb{N^{+}}$, all shortest-paths between $u\in N_v^{h}(G)$ and $w \in N_v^{h-s}(G)$ on $G(V\setminus\{v\})$ that satisfy $dis_{G(V\setminus \{v\})}(u,w)\leq h$ are contained in the induced subgraph $G(N_v^{h}(G))$, where $s=dis_G(u,v)$. In other words, for any shortest path $P=(u,...,w_i,...,w)$ between $u$ and $w$ on $G(V\setminus\{v\})$, we have $w_i \in N_v^{h}(G)$ for all $w_i \in P$.
\end{theorem}
\begin{proof}
Suppose, to the contrary, that there exists a shortest-path $P=(u,...,w',...,w)$ between $u \in N_v^{h}(G)$ and $w \in N_v^{h-s}(G)$ on $G(V\setminus\{v\})$ that satisfies $w' \notin N_v^{h}(G)$. By this assumption, we have  $dis_{G(V\setminus\{v\})}(u,w) = dis_{G(V\setminus\{v\})}(u,w') + dis_{G(V\setminus\{v\})}(w',w)$. Then, $dis_G(v, w') - dis_G(v, u) \le dis_G(u, w') \le dis_{G(V\setminus\{v\})}(u,w')$ holds by triangle inequality. Since $w' \notin N_v^{h}(G)$ (by assumption), we have $dis_G(v, w')>h$. Thus, we have $h-s < dis_{G(V\setminus\{v\})}(u,w')$. Similarly, we have $dis_G(v, w')-dis_G(v, w) \le dis_G( w', w) \le dis_{G(V\setminus\{v\})}(w',w)$.  Therefore, we get that $s= h-(h-s) < dis_{G(V\setminus\{v\})}(w',w)$. Putting it all together, we can derive that $h < dis_{G(V\setminus\{v\})}(u,w) $ which is a contradiction.
\end{proof}
